# Supplementary material for: Nonlocal Structural Effects of Water on DNA Homology Recognition
Source: arXiv:2402.03213 ancillary file (2024-03-07)
Supplement: Supplementary file 1 [file Supplemental_Material.pdf]

**Supplemental Material**

# Nonlocal Structural Effects of Water on DNA Homology Recognition

**Ehud Haimov, Jonathan G. Hedley, Alexei A. Kornyshev**

## 1. Non-local electrostatic interaction energy between two parallel dsDNA molecules

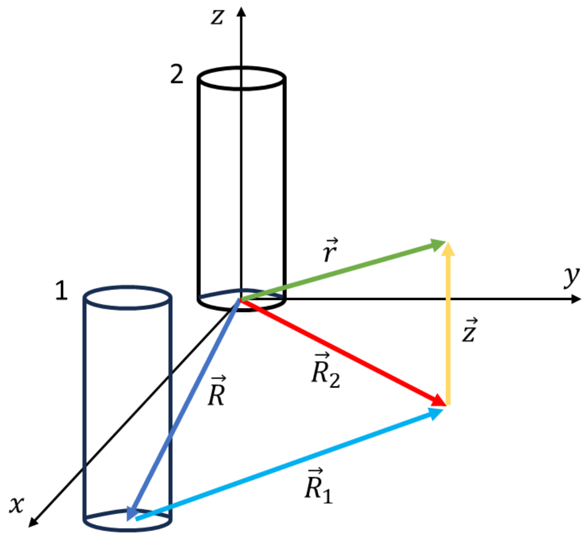


**Figure 1**: Description of system's geometry. The cylinders represent the molecules. $\vec{R}$, $\vec{R}_1$ and $\vec{R}_2$ are all contained in the same $XY$ plane.

Let us first consider the general case of two cylindrical molecules, numbered 1 and 2, situated parallel to each other at a center-to-center distance $R$, as depicted in Fig. 1. Each molecule is characterized by a non-uniform cylindrical surface charge distribution at a distance $a$ from its center, and an impenetrable dielectric core at a different distance $b < a$ from the center of the molecule.

The total charge distribution for each molecule contains two contributions, the first is due to physical charges, and the second is due to image charges. Image charges are induced due to a change in dielectric environment between the liquid and impenetrable core. The total charge distribution of each molecule $\nu$ expressed in its own cylindrical system, is given by

$$\rho_\nu^{(\mathrm{tot})}(\vec{r}) = \sigma_\nu(z,\varphi)\delta(R_\nu - a) + \rho_\nu^{(\mathrm{im})}(\vec{r});\ \nu = 1, 2$$

$\rho_\nu^{(\mathrm{im})}$ is the charge distribution due to image charges which are situated inside the impenetrable core.

Here we adopted the Debye-Bjerrum approximation that all charges, both phosphates strands and adsorbed specific counterions, sit at the same distance $a$ from each molecule's center.

Let us start by defining aspects in the geometry of our system. We define $\vec{r}$ as a position vector stretched from the origin situated at the center of the bottom base of cylinder #2. The position vector can be decomposed as:

$$\vec{r} = \vec{R}_2 + \vec{z}. \tag{1}$$

where $\vec{R}_2$ is a planar radial vector and $\vec{z}$ is along the long axis. We can also write the position vector $\vec{r}$ in terms of $\vec{R}_1$, a planar radial vector stretched from the center of the bottom base of molecule #1 until the head of $\vec{R}_2$, as:

$$\vec{r} = \vec{R} + \vec{R}_1 + \vec{z}, \tag{2}$$

where $\vec{R}$ is a planar radial vector pointing from the center of the base of the first to the second cylinder, as depicted in Fig. 1.

The electrostatic interaction between two charged bodies is generally given by:

$$U = \int_{\rho_1 \neq 0} \Phi_2^{(\mathrm{tot})}(\vec{r})\rho_1^{(\mathrm{tot})}(\vec{r})\mathrm{d}^3\vec{r} \tag{3}$$

where $\Phi_2$ is the potential molecule 2 creates, and $\rho_1$ is the volumetric charge density of molecule 1.

The Fourier transform $\tilde{f}(\vec{k})$ and its inverse $f(\vec{r})$ for a general function is defined as:

$$\tilde{f}(\vec{k}) = \int \mathrm{d}^3\vec{r} e^{-i\vec{k}\cdot\vec{r}} f(\vec{r}) \tag{4}$$

$$f(\vec{r}) = \frac{1}{(2\pi)^3}\int \mathrm{d}^3\vec{k} e^{i\vec{k}\cdot\vec{r}}\tilde{f}(\vec{k}). \tag{5}$$

Writing $\Phi_2(\vec{r})$ and $\rho_1(\vec{r})$ as inverse transforms in Eq. (3) we get:

$$U = \frac{1}{(2\pi)^6}\int \mathrm{d}^3\vec{r} \int \tilde{\Phi}_2^{(\mathrm{tot})}(\vec{k}) e^{i\vec{k}\cdot\vec{r}}\mathrm{d}^3\vec{k} \int \tilde{\rho}_1^{(\mathrm{tot})}(\vec{k}') e^{i\vec{k}'\cdot\vec{r}}\mathrm{d}^3\vec{k}' \tag{6}$$

using $\int e^{i(\vec{k}+\vec{k}')\cdot\vec{r}}\mathrm{d}^3\vec{r} = (2\pi)^3\delta(\vec{k}+\vec{k}')$ we get,

$$U = \frac{1}{(2\pi)^3}\int \tilde{\Phi}_2^{(\mathrm{tot})}(\vec{k})\tilde{\rho}_1^{(\mathrm{tot})}(-\vec{k})\mathrm{d}^3\vec{k} \tag{7}$$

The task has now been reduced to finding $\tilde{\rho}_1^{(\mathrm{tot})}, \tilde{\Phi}_2^{(\mathrm{tot})}$ and solving the integral in Eq. (7).

The relation between potential and charge distribution in electrolyte medium (outside the cores) is determined by the specific electrostatic interaction mediated by the electrolyte response. First, without getting into a specific electrolyte response model, we can describe the overall linear interaction by a general Green's function $G(\vec{r}, \vec{r}')$, such that:

$$\Phi_2^{(\mathrm{tot})}(\vec{r}) = \int G(\vec{r}, \vec{r}')\rho_2^{(\mathrm{tot})}(\vec{r}')\mathrm{d}^3\vec{r}' \tag{8}$$

Assuming homogenous media, $G(\vec{r}, \vec{r}') = G(\vec{r} - \vec{r}')$, consequently yielding the following relation in Fourier space:

$$\tilde{\Phi}_2^{(\mathrm{tot})}(\vec{k}) = \tilde{G}(\vec{k})\tilde{\rho}_2^{(\mathrm{tot})}(\vec{k}) = \tilde{G}(\vec{k})\left(\tilde{\rho}_2(\vec{k}) + \tilde{\rho}_2^{(\mathrm{im})}(\vec{k})\right). \tag{9}$$

To go any further with Eq. (9), one must find $\tilde{\rho}_2(\vec{k})$ explicitly. Considering only the dominant term in for the image charge, we have the following distribution in $\vec{r}$-space:

$$\rho_2^{(\mathrm{tot})}(\vec{r}) = \sigma_2(\varphi_2, z)\delta(R_2 - a) + \sigma_2^{(\mathrm{im})}(\varphi_2, z)\delta(R_2 - b^-) \tag{10}$$

where $b^- = b - \Delta$, where $\frac{\Delta}{b} \ll 1$. The variable $z$ is considered the same for all systems, thus there is no need to give it a subscript. The Fourier transform of the first term in Eq. (10) is given by:

$$\tilde{\rho}_2(\vec{k}) = \int \sigma_2(\varphi_2, z)\delta(R_2 - a)e^{-i\vec{k}\cdot\vec{r}}R_2 dR_2 d\varphi_2 dz \tag{11}$$

where $(R_2, \varphi_2, z)$ are the cylindrical coordinates of molecule 2. We can immediately solve the integral in Eq. (11) over $R_2$ and get,

$$\tilde{\rho}_2(\vec{k}) = a\int \sigma_2(\varphi_2, z)e^{-iKa\cos\left(\varphi_{\vec{K}} - \varphi_2\right)}e^{-iqz}d\varphi_2 dz \tag{12}$$

where we denoted the cylindrical wavelength vector as $\vec{K} = k_x\hat{x} + k_y\hat{y}$ , the z-axis component of the wavelength $q = k_z$, and the cylindrical angle of $\vec{K}$ as $\varphi_{\vec{K}} = \arctan(k_y/k_x)$.

Since the surface charge distribution of the second molecule, $\sigma_2(\varphi_2, z)$, is a periodic function of the angle coordinate $\varphi_2$, its inverse Fourier transform is expressed by:

$$\sigma_2(\varphi_2, z) = \frac{1}{(2\pi)^2}\sum_{m=-\infty}^{\infty}\int_{-\infty}^{\infty}\tilde{\sigma}_2(m, q')e^{im\varphi_2}e^{iq'z}dq' \tag{13}$$

Plugging Eq. (13) into Eq. (12), and using the identity $\int_{-\infty}^{\infty} dz e^{i(q'-q)z} = 2\pi\delta(q' - q)$, we get:

$$\tilde{\rho}_2(\vec{k}) = \frac{a}{2\pi}\sum_{m=-\infty}^{\infty}\tilde{\sigma}_2(m, q)\int_0^{2\pi} e^{-iKa\cos\left(\varphi_{\vec{K}} - \varphi_2\right)}e^{im\varphi_2}d\varphi_2 \tag{14}$$

Substituting variables $\theta = \varphi_2 - \varphi_{\vec{K}}$ we get:

$$\tilde{\rho}_2(\vec{k}) = \frac{a}{2\pi}\sum_{m=-\infty}^{\infty}\tilde{\sigma}_2(m, q)e^{im\varphi_{\vec{K}}}\int_{-\varphi_{\vec{K}}}^{-\varphi_{\vec{K}}+2\pi} e^{im\theta}e^{-iKa\cos\theta}d\theta \tag{15}$$

Since the integrand is $2\pi$ periodic in $\theta$, and since the integration limits are over a full period, it doesn't matter over which full period we integrate over. Thus, for the sake of simplicity we may instead change the limits to be from $0$ to $2\pi$. That way the integral aligns with Bessel's first integral identity $\int_0^{2\pi} e^{\pm im\theta}e^{-iKa\cos\theta}d\theta = (-1)^m 2\pi i^m J_m(Ka)$. Using this identity in Eq. (15), we get,

$$\tilde{\rho}_2(\vec{k}) = a\sum_{m=-\infty}^{\infty}\tilde{\sigma}_2(m, q)(-1)^m i^m J_m(Ka)e^{im\varphi_{\vec{K}}} \tag{16}$$

Following the same procedure for the second term in Eq. (10), and plugging the result into Eq. (9), we arrive at the transformed potential created by molecule 2:

$$\tilde{\Phi}_2^{(\mathrm{tot})}(K, \varphi_{\vec{K}}, q) = \tilde{G}(K, \varphi_{\vec{K}}, q)\sum_{m=-\infty}^{\infty}(-1)^m i^m\left[a\tilde{\sigma}_2(m, q)J_m(Ka) + b^-\tilde{\sigma}_2^{(\mathrm{im})}(m, q)J_m(Kb^-)\right]e^{im\varphi_{\vec{K}}} \tag{17}$$

Which inverse transform gives,

$$\Phi_2^{(\mathrm{tot})}(R_2,\varphi_2,z) = \frac{1}{(2\pi)^3}\int_{-\infty}^{\infty} dq \int_0^{\infty} K\, dK \int_0^{2\pi} d\varphi_{\vec{K}}\; e^{iqz} e^{iKR_2\cos\left(\varphi_{\vec{K}}-\varphi_2\right)} \tilde{G}\left(K,\varphi_{\vec{K}},q\right)$$
$$\times \sum_{m=-\infty}^{\infty} (-1)^m i^m \left[a\tilde{\sigma}_2(m,q)J_m(Ka) + b^{-}\tilde{\sigma}_2^{(\mathrm{im})}(m,q)J_m(Kb^{-})\right] e^{im\varphi_{\vec{K}}}$$

(18)

To make further progress with the integral presented in Eq. (18), the framework of the model needs further specification. We assume that the medium is isotropic, i.e., $G(\vec{r}-\vec{r}') = G(|\vec{r}-\vec{r}'|)$ and, as a consequence, $\tilde{G}(\vec{k}) = \tilde{G}(|\vec{k}|) = \tilde{G}(\sqrt{K^2+q^2})$, independent of $\varphi_{\vec{K}}$. The integration in Eq. (18) over $\varphi_{\vec{K}}$ therefore gives:

$$\Phi_2^{(\mathrm{tot})}(R_2,\varphi_2,z) = \frac{1}{(2\pi)^2}\int_{-\infty}^{\infty} dq \int_0^{\infty} K\, dK\, e^{iqz}\tilde{G}\left(\sqrt{K^2+q^2}\right) \times \sum_{m=-\infty}^{\infty}\left[a\tilde{\sigma}_2(m,q)J_m(Ka) + b^{-}\tilde{\sigma}_2^{(\mathrm{im})}(m,q)J_m(Kb^{-})\right]J_m(KR_2)e^{im\varphi_2} \quad (19)$$

where we used $\int_0^{2\pi} e^{\pm im\theta} e^{iKa\cos\theta} d\theta = 2\pi i^m J_m(Ka)$.

Defining $\tilde{\Phi}_2^{(\mathrm{tot})}(R_2,m,q)$ through $\Phi_2^{(\mathrm{tot})}(R_2,\phi_2,z) = \frac{1}{(2\pi)^2}\sum_m \int dq\, \tilde{\varphi}_2^{(\mathrm{tot})}(R_2,m,q) e^{im\phi_2} e^{iqz}$, we obtain:

$$\Phi_2^{(\mathrm{tot})}(R_2,m,q) = a\tilde{\sigma}_2(m,q)\int_0^{\infty} KdK\; \tilde{G}\left(\sqrt{K^2+q^2}\,\right)J_m(Ka)J_m(KR_2) + b^{-}\tilde{\sigma}_2^{(\mathrm{im})}(m,q)\int_0^{\infty} KdK\; \tilde{G}\left(\sqrt{K^2+q^2}\,\right)J_m(Kb^{-})J_m(KR_2) \quad (20)$$

To account for the boundary conditions at the hydrophobic core, we proceed to calculate the potential in Eq. (20) for the region $b < R_2 < a$. For brevity and future use, let's define the following auxiliary function:

$$\mathcal{A}_m(x,R_2,q) = \int_0^{\infty} KdK\; \tilde{G}\left(\sqrt{K^2+q^2}\,\right)J_m(Kx)J_m(KR_2) \quad (21)$$

It should be noted that the integral in Eq. (21) may produce a different analytical solution depending on whether $x < R_2$ or $x > R_2$.

Substituting Eq. (21) into Eq. (20) we get:

$$\Phi_2^{(\mathrm{tot})}(R_2,m,q)\Big|_{b<R_2<a} = a\tilde{\sigma}_2(m,q)\mathcal{A}_m(a,R_2,q) + b\tilde{\sigma}_2^{(\mathrm{im})}(m,q)\mathcal{A}_m(b,R_2,q) \quad (22)$$

Where we made the approximation $b^{-} \approx b$.

Potential inside the core is governed by Poisson equation, which gives:

$$\Phi_2^{(\mathrm{tot})}(R_2,m,q)\Big|_{R_2<b} = B(q,m)I_m(|q|R_2) \quad (23)$$

So that overall:

$$\Phi_2^{(\mathrm{tot})}(R_2 < a, m, q) =$$
$$\begin{cases} B(q,m) I_m(|q|R_2) & R_2 < b \\ a\tilde{\sigma}_2(m,q)\mathcal{A}_m(a,R_2,q) + b\tilde{\sigma}_2^{(\mathrm{im})}(m,q)\mathcal{A}_m(b,R_2,q) & b < R_2 < a \end{cases} \tag{24}$$

Boundary conditions read as:

$$\Phi_2^{(\mathrm{tot})}(b^+, m, q) = \Phi_2^{(\mathrm{tot})}(b^-, m, q) \tag{25}$$

$$\epsilon^* \frac{\partial \Phi_2}{\partial R_2}\bigg|_{R_2=b^+} = \epsilon_c \frac{\partial \Phi_2}{\partial R_2}\bigg|_{R_2=b^-} \tag{26}$$

From the continuity of potential (first boundary condition) we get:

$$B(q,m) = \frac{a\tilde{\sigma}_2(m,q)\mathcal{A}_m(a,b,q) + b\tilde{\sigma}_2^{(\mathrm{im})}(m,q)\mathcal{A}_m(b,b,q)}{I_m(|q|b)} \tag{27}$$

From the second boundary condition we get the ratio between real and imaginary charge densities:

$$\Xi(m,q) = \frac{\tilde{\sigma}_2^{(\mathrm{im})}(m,q)}{\tilde{\sigma}_2(m,q)} = -\frac{a}{b}\frac{\mathcal{A}'_m(a,b,q) - \gamma|q|\frac{I'_m(|q|b)}{I_m(|q|b)}\mathcal{A}_m(a,b,q)}{\mathcal{A}'_m(b,b,q) - \gamma|q|\frac{I'_m(|q|b)}{I_m(|q|b)}\mathcal{A}_m(b,b,q)} \tag{28}$$

where $\gamma \equiv \frac{\epsilon_c}{\epsilon^*}$, and $\mathcal{A}'_m = \partial\mathcal{A}_m/\partial R_2$.

Plugging Eq. (17) into Eq. (7) we get:

$$U = \frac{1}{(2\pi)^3}\int \tilde{G}\left(\sqrt{K^2+q^2}\right)\sum_{m=-\infty}^{\infty}(-1)^m i^m \tilde{\sigma}_2(m,q)[aJ_m(Ka) + b\Xi(m,q)J_m(Kb)]e^{im\phi_{\vec{K}}}\,\tilde{\rho}_1^{(\mathrm{tot})}(-\vec{k})\mathrm{d}^3\vec{k} \tag{29}$$

Where, by definition,

$$\tilde{\rho}_1^{(\mathrm{tot})}(-\vec{k}) = \int \mathrm{d}^3\vec{r} e^{i\vec{k}\cdot\vec{r}}\rho_1^{(tot)}(\vec{r}) \tag{30}$$

To proceed in calculation $\tilde{\rho}_1^{(\mathrm{tot})}(-\vec{k})$, we now introduce the other cylindrical system centered around molecule 1. We can write the position vector using this coordinate system by making use of Eq. (2):

$$\tilde{\rho}_1^{(\mathrm{tot})}(-\vec{k}) = e^{i\vec{K}\cdot\vec{R}}\tilde{\tilde{\rho}}_1^{(tot)}(-\vec{k}) \tag{31}$$

where $\tilde{\tilde{\rho}}_1^{(tot)} = \int R_1 dR_1 d\varphi_1 dz\; e^{i\vec{K}\cdot\vec{R}_1}e^{iqz}\rho_1^{(tot)}(\vec{r})$.

it should be clear that we can use any volumetric element to integrate over, we specifically use that of the cylindrical system of molecule 1.

As with the second molecule, we will decompose the total charge density of the first molecule into real charge and image charge:

$$\tilde{\tilde{\rho}}_1^{(tot)}(-\vec{k}) = \tilde{\tilde{\rho}}_1(-\vec{k}) + \tilde{\tilde{\rho}}_1^{(\mathrm{im})}(-\vec{k}) \tag{32}$$

From here, we just repeat the procedure that was done for the second molecule, only now we do it for $\tilde{\tilde{\rho}}_1^{(tot)}(-\vec{k})$. After redoing the same procedure, we get:

$$\tilde{\tilde{\rho}}_1^{(\mathrm{tot})}(-\vec{k}) = \sum_{n=-\infty}^{\infty} i^n\left[a\tilde{\sigma}_1(-n,-q)J_n(Ka) + b\tilde{\sigma}_1^{(\mathrm{im})}(-n,-q)J_n(Kb)\right]e^{-in\varphi_{\vec{K}}} \tag{33}$$

Plugging Eqs. (31) and (33) into Eq. (29) we get:

$$U = \frac{1}{(2\pi)^3}\int e^{iKR\cos\varphi_{\vec{K}}}\tilde{G}\left(\sqrt{K^2+q^2}\right)\sum_{n,m=-\infty}^{\infty} e^{i(m-n)\varphi_{\vec{K}}}i^{m+n}(-1)^m\tilde{\sigma}_1(-n,-q)\tilde{\sigma}_2(m,q)[aJ_m(Ka) + b\Xi(m,q)J_m(Kb)]\,[aJ_n(Ka) + b\Xi(-n,-q)J_n(Kb)]KdKd\varphi_{\vec{K}}dq \tag{34}$$

Isolating the integral over $\varphi_{\vec{K}}$ and once again using $\int_0^{2\pi} e^{\pm i(m-n)\theta}e^{ix\cos\theta}d\theta = 2\pi i^{m-n}J_{m-n}(x)$

$$U = \frac{1}{(2\pi)^2}\int \tilde{G}\left(\sqrt{K^2+q^2}\right)\sum_{n,m=-\infty}^{\infty}J_{m-n}(KR)\tilde{\sigma}_1(-n,-q)\tilde{\sigma}_2(m,q)[aJ_m(Ka) + b\Xi(m,q)J_m(Kb)]\,[aJ_n(Ka) + b\Xi(-n,-q)J_n(Kb)]KdKdq \tag{35}$$

Using $J_{-\nu}(z) = (-1)^\nu J_\nu(z)$ we get:

$$U = \frac{1}{(2\pi)^2}\int \tilde{G}\left(\sqrt{K^2+q^2}\right)\sum_{n,m=-\infty}^{\infty}(-1)^{n-m}J_{n-m}(KR)\tilde{\sigma}_1(-n,-q)\tilde{\sigma}_2(m,q)[aJ_m(Ka) + b\Xi(m,q)J_m(Kb)]\,[aJ_n(Ka) + b\Xi(-n,-q)J_n(Kb)]KdKdq \tag{36}$$

Expanding the square brackets:

$$U = \frac{1}{(2\pi)^2}\sum_{n,m=-\infty}^{\infty}(-1)^{n-m}\int_{-\infty}^{\infty}dq\ \tilde{\sigma}_1(-n,-q)\tilde{\sigma}_2(m,q)\ \int_0^{\infty}KdK\ \tilde{G}\left(\sqrt{K^2+q^2}\right)\times$$
$$[a^2J_{n-m}(KR)J_n(Ka)J_m(Ka) + ab\Xi(m,q)J_{n-m}(KR)J_n(Ka)J_m(Kb) +$$
$$ab\Xi(-n,-q)J_{n-m}(KR)J_n(Kb)J_m(Ka) + b^2\Xi(-n,-q)\Xi(m,q)J_{n-m}(KR)J_n(Kb)J_m(Kb)] \tag{37}$$

Defining $\Omega_{n,m}(q,x,y,z) = yz\int_0^{\infty}K\,dK\ \tilde{G}\left(\sqrt{K^2+q^2}\right)J_{n-m}(Kx)J_n(Ky)J_m(Kz)$, we can rewrite the expression above as:

$$U = \frac{1}{(2\pi)^2}\sum_{n,m=-\infty}^{\infty}(-1)^{n-m}\int_{-\infty}^{\infty}dq\ \tilde{\sigma}_1(-n,-q)\tilde{\sigma}_2(m,q)\ \times\left[\Omega_{n,m}(q,R,a,a)\ + \Xi(m,q)\Omega_{n,m}(q,R,a,b) + \Xi(-n,-q)\Omega_{n,m}(q,R,b,a) + \Xi(-n,-q)\Xi(m,q)\Omega_{n,m}(q,R,b,b)\right] \tag{38}$$

For conciseness, let us define:

$$\mathcal{W}_{n,m}(q,R,a,b) = \Omega_{n,m}(q,R,a,a)\ + \Xi(m,q)\Omega_{n,m}(q,R,a,b) + \Xi(-n,-q)\Omega_{n,m}(q,R,b,a) + \Xi(-n,-q)\Xi(m,q)\Omega_{n,m}(q,R,b,b) \tag{39}$$

which makes the result above much more compact:

$$u = \frac{1}{(2\pi)^2}\sum_{n,m=-\infty}^{\infty}(-1)^{n-m}\int_{-\infty}^{\infty}dq\ \tilde{\sigma}_1(-n,-q)\tilde{\sigma}_2(m,q)\,\mathcal{W}_{n,m}(q,R,a,b) \tag{40}$$

Since we consider infinite molecules in parallel, and since there are charges throughout the whole length, i.e. even at ‘infinity’ (like in the case of DNA), the total interaction energy of the system diverges. For that reason, it makes sense to consider the interaction energy per unit length:

$$u \equiv \lim_{L\to\infty}\frac{U}{L} = \lim_{L\to\infty}\frac{1}{(2\pi)^2}\sum_{n,m=-\infty}^{\infty}(-1)^{n-m}\int dq\ \mathcal{W}_{n,m}(q,R,a,b)\frac{\tilde{\sigma}_1(-q,-n)\tilde{\sigma}_2(q,m)}{L} \tag{41}$$

Considering symmetry arguments, we can rewrite the above as:

$$u = \frac{1}{(2\pi)^2}\sum_{n,m=-\infty}^{\infty}(-1)^{n-m}\int dq\ \mathcal{W}_{n,m}(q,R,a,b)\mathcal{S}_{12}(q,n,m) \tag{42}$$

where we defined the surface charge density pair correlation function $\mathcal{S}_{12}$ as:

$$\mathcal{S}_{12}(q,n,m) = \lim_{L\to\infty}\left\{\frac{\tilde{\sigma}_1(-q,-n)\tilde{\sigma}_2(q,m)+\tilde{\sigma}_1(q,n)\tilde{\sigma}_2(-q,-m)}{2L}\right\} \tag{43}$$

Eqs. (40-43) refer to the interaction between any two cylindrical molecules with an impenetrable core and general charge distributions. Let us next focus on the specific case of ds-DNA molecules.

## 2. Calculation of $\mathcal{S}_{12}(q,n,m)$ for Double Helices with condensed counterion distributions

The total charge distribution is given by $\sigma = \sigma^{\mathrm{DNA}} + \sigma^{\mathrm{CC}}$, where CC describes the condensed counterions. In general, for any N-stranded, right-handed helical surface charge distribution, we can write $\sigma_{\mathrm{N-helix}}(z,\varphi)$ as

$$\sigma_{\mathrm{N-helix}}(z,\varphi) = \frac{2\pi\bar{\sigma}}{N}\sum_{i=0}^{N}\delta\big(\varphi - \phi_i - g(z-z_i)\big) \tag{44}$$

where $(\phi_i, z_i)$ characterizes the coordinates of each individual helical strand, $i$ . It is clear here that these strands are modelled as infinitely thin. In this document, as we are deriving an expression for any arbitrary linear response function, we need to generalize this charge distribution. This can be done by introducing a form factor, $\psi(z,\phi)$, over which we smear $\sigma$ such that

$$\sigma_{\mathrm{smeared}}(z,\varphi) = \int_0^{2\pi} d\varphi' \int_{-\infty}^{\infty} dz'\ \psi(z-z',\varphi-\varphi')\sigma(z',\varphi') \tag{45}$$

Hence, for a double helix, we can write

$$\sigma_\nu^{\mathrm{DNA}}(z,\varphi_\nu) = \pi\bar{\sigma}_\nu\sum_{i=1}^{2}\int_0^{2\pi} d\varphi' \int_{-\infty}^{\infty} dz'\ \psi(z-z',\varphi_\nu-\varphi_\nu{}')\delta\left(\varphi_\nu{}' - \phi_{\nu,i} - g\big(z'-z_{\nu,i}\big)\right) \tag{46}$$

where $\nu = 1,2$ labels the DNA molecules and $i = 1,2,\ldots,N$ labels the individual helical strands in each molecule. Focusing on the case of ds-DNA, i.e. $N = 2$ and taking the Fourier transform we get:

$$\tilde{\sigma}_\nu^{\mathrm{DNA}}(q,n) = \int_0^{2\pi} d\varphi_\nu \int_{-\infty}^{\infty} dz\ \sigma_\nu(z,\varphi_\nu)e^{-iqz}e^{-in\varphi_\nu}$$

$$= \pi\bar{\sigma}_\nu\sum_{i=1}^{2}\int_0^{2\pi} d\varphi \int_{-\infty}^{\infty} dz\ e^{-iqz}e^{-in\varphi_\nu}\int_{-\infty}^{\infty} dz'\ \psi_\nu\left(z-z',\varphi_\nu-\left(\phi_{\nu,i}+g\big(z'-z_{\nu,i}\big)\right)\right)$$

$$= \pi\bar{\sigma}_\nu\sum_{i=1}^{2}\int_{-\infty}^{\infty} dz\int_{-\infty}^{\infty} dz'\ e^{-in\left(\phi_{\nu,i}+g(z'-z_{\nu,i})\right)}e^{-iqz}\int_0^{2\pi} d\phi\ e^{-in\left(\varphi_\nu-\left(\phi_{\nu,i}+g(z'-z_{\nu,i})\right)\right)}\psi_\nu\left(z-z',\varphi_\nu-\left(\phi_{\nu,i}+g\big(z'-z_{\nu,i}\big)\right)\right) \tag{47}$$

We see that the integral over $\varphi_\nu$ is the Fourier transform:

$$\int_0^{2\pi} d\varphi_v\, e^{-in\left(\varphi_v-\left(\phi_{v,i}+g(z'-z_{v,i})\right)\right)}\psi_v\left(z-z',\phi-\left(\phi_{v,i}+g\left(z'-z_{v,i}\right)\right)\right)=\psi_v(z-z',n) \quad (48)$$

Therefore:

$$\tilde{\sigma}_v^{\mathrm{DNA}}(q,n)=\pi\bar{\sigma}_v\sum_{i=1}^{2} e^{-in\phi_{v,i}}e^{ingz_{v,i}}\int_{-\infty}^{\infty}dz\int_{-\infty}^{\infty}dz'\,e^{-ingz'}e^{-iqz}\psi_v(z-z',n)$$

$$=\pi\bar{\sigma}_v\sum_{i=1}^{2} e^{-in\phi_{v,i}}e^{ingz_{v,i}}\int_{-\infty}^{\infty}dz'\,e^{-ingz'}e^{-iqz'}\int_{-\infty}^{\infty}dz\,e^{-iq(z-z')}\psi_v(z-z',n)$$

$$=\pi\bar{\sigma}_v\sum_{i=1}^{2} e^{-in\phi_{v,i}}e^{ingz_{v,i}}\,\tilde{\psi}_v(q,n)\int_{-\infty}^{\infty}dz'\,e^{ing(z'-z_{v,i})}e^{-iqz'}$$
$$=2\pi^2\bar{\sigma}_v\sum_{i=1}^{2} e^{-in\phi_{v,i}}e^{ingz_{v,i}}\,\tilde{\psi}_v(q,n)\delta(q+ng) \quad (49)$$

The helicity of the strands is already taken into account by the delta function, however, the angle of the position vector at $z=0$ needs to be defined as a reference angle. For each strand we define the angle of the position vector at $z=0$ as: $\phi_{v,i}(z_{v,i}=0)=\phi_v(z_{v,i}=0)\pm\phi_s/2$. For brevity, from this point on, we refer to $\phi_v(z_{v,i}=0)$ as $\phi_v$, where $\phi_v$ is the angle the vector that points along the centre of the minor groove makes with the $x$ axis at $z=0$:

$$\tilde{\sigma}_v^{\mathrm{DNA}}(q,n)=2\pi^2\bar{\sigma}_v\tilde{\psi}_v(q,n)\delta(q+ng)\left[e^{-in\phi_s/2}+e^{in\phi_s/2}\right]e^{-in\phi_v}$$

$$=4\pi^2\bar{\sigma}_v\tilde{\psi}_v(q,n)\delta(q+ng)\cos\left[\frac{n\phi_s}{2}\right]e^{-in\phi_v} \quad (50)$$

For the form factor, $\psi(z,\varphi)$ is normalised such that $\int\int\psi(z,\varphi)d\varphi dz=1$. Hence, $\tilde{\psi}(q=0,n=0)=\int\int\psi(z,\varphi)d\varphi dz=1$. For the condensed counterion distributions, we follow a similar method, where we define:

$$\sigma_v^{CC}(z,\varphi_v)=2\pi\bar{\sigma}_c\int_{-\infty}^{\infty}dz'\,\Psi_{\mathrm{CC},v}(z-z')\delta(\varphi_v-\phi_v-gz') \quad (51)$$

Where $\Psi_{CC,v}(z-z')$ denotes a specific smeared counterion adsorption pattern along the DNA molecule. In a similar way, we use the Fourier transform:

$$\tilde{\sigma}_v^{\mathrm{CC}}(q,n)=\int_0^{2\pi}d\varphi_v\int_{-\infty}^{\infty}dz\;\sigma_v^{\mathrm{CC}}(z,\varphi_v)e^{-iqz}e^{-in\varphi_v}$$

$$=2\pi\bar{\sigma}_c\int_0^{2\pi}d\varphi_v\int_{-\infty}^{\infty}dz\int_{-\infty}^{\infty}dz'\,\Psi_{\mathrm{CC},v}(z-z')\delta(\varphi_v-\phi_v-gz')\,e^{-iqz}e^{-in\varphi_v}$$

$$=2\pi\bar{\sigma}_c\,e^{-in\phi_v}\int_{-\infty}^{\infty}dz'\,e^{-iqz'}e^{-ingz'}\int_{-\infty}^{\infty}dz\,\Psi_{\mathrm{CC},v}(z-z')e^{-iq(z-z')}$$

$$=4\pi^2\bar{\sigma}_c\,\delta(q+ng)\tilde{\Psi}_{\mathrm{CC},v}(q)e^{-in\phi_v} \quad (52)$$

We can write $\Psi_{\mathrm{CC}}(z)$, as a convolution between some smearing form factor function $\psi_{\mathrm{CC}}$ and an adsorption pattern $p(z)$ such that

$$\Psi_{CC}(z)=\int_{-\infty}^{\infty}dz'\psi_{CC}(z-z')p(z) \quad (53)$$

For $p(z)$, we use the 4-state counterion adsorption pattern, written as

$$p(z)=f_1\delta(z)+f_2\delta\left(z-\frac{H}{2}\right)+\frac{f_3}{2}\left\{\delta\left(z-\frac{H\phi_s}{4\pi}\right)+\delta\left(z+\frac{H\phi_s}{4\pi}\right)\right\}+\frac{2\pi}{L}f_4 \quad (54)$$

where $f_1$ corresponds to the minor groove, $f_2$ corresponds to the major groove, $f_3$ corresponds to the strands, and $f_4$ is a smeared counterion cloud over the entire cylinder. For simplicity, if we assume that all sites are smeared with the same $\psi_{CC}$, we can write:

$$\tilde{p}(q)=\tilde{\psi}_{\mathrm{CC}}(q)\left(f_1+f_2(-1)^n+f_3\cos\left(\frac{n\phi_s}{2}\right)+\frac{2\pi}{L}f_4\delta(q)\right) \quad (55)$$

Therefore, we can write the counterion distributions as

$$\tilde{\sigma}_v^{\mathrm{CC}}(q,n)=4\pi^2\bar{\sigma}_c\,\delta(q+ng)\tilde{\psi}_{\mathrm{CC}}\left[\left(f_1+f_2(-1)^n+f_3\cos\left(\frac{n\phi_s}{2}\right)\right)+\frac{2\pi}{L}f_4\delta(q)\right]e^{-in\phi_v} \quad (56)$$

Using $\bar{\sigma}_c = -\Theta\bar{\sigma}$, we can write for the full charge distribution:

$$\tilde{\sigma}_\nu(q,n) = 4\pi^2\bar{\sigma}\delta(q+ng)e^{-in\phi_\nu}\tilde{P}_\nu(q)e^{-in\phi_\nu} \tag{57}$$

where

$$\tilde{P}_\nu(q) = \tilde{\psi}_\nu(q,n)\cos\left[\frac{n\phi_s}{2}\right] - \Theta\tilde{\psi}_{CC}(q)\left(f_1 + f_2(-1)^n + f_3\cos\left(\frac{n\phi_s}{2}\right)\right) - \frac{2\pi}{L}\Theta f_4\delta(q) \tag{58}$$

$$= \left(e^{-\frac{1}{2}n^2g^2\Delta_\mathrm{v}^2} - \Theta f_3 e^{-\frac{1}{2}n^2g^2\Delta_\mathrm{c}^2}\right)\cos\left(\frac{n\phi_s}{2}\right) - \Theta e^{-\frac{1}{2}n^2g^2\Delta_\mathrm{c}^2}(f_1 + f_2(-1)^n) - \frac{2\pi}{L}\Theta f_4\delta(q) \tag{59}$$

Despite deriving this general result with form factors, later on in this work we use a simple Lorentzian type Green's function, where smearing will not result in any major modifications to the results. Such an effect is expected to be important only when overresponding nonlocal Green's functions are considered. In these cases, the form factors will smear out the overresponse to the infinitesimally thin charge distribution , a necessary detail to obtain a more physical picture. Hence in this work, we simply set $\tilde{\psi}_\nu(q,n) = \tilde{\psi}_{CC}(q) = 1$.

Using the above, and plugging into $S_{12}(q,n,m)$, we need to calculate the products:

$$\tilde{\sigma}_1(-q,-n)\tilde{\sigma}_2(q,m) = 16\pi^4\bar{\sigma}^2\delta(q+ng)\delta(q+mg)\tilde{P}_1(-q)\tilde{P}_2(q)e^{in\phi_1}e^{-im\phi_2} \tag{60}$$

$$\tilde{\sigma}_1(q,n)\tilde{\sigma}_2(-q,-m) = 16\pi^4\bar{\sigma}^2\delta(q+ng)\delta(q+mg)\tilde{P}_1(q)\tilde{P}_2(-q)e^{-in\phi_1}e^{im\phi_2} \tag{61}$$

We use:

$$\delta_{q,-ng} = \lim_{L\to\infty}\frac{2\pi\delta(q+ng)}{L}\ ,$$

and $\tilde{P}_1(q) = \tilde{P}_2(-q)$, to obtain:

$$\mathcal{S}_{12}(q,n,m) = 8\pi^3\bar{\sigma}^2\cos[n\phi_1 - m\phi_2]\,\tilde{P}(q)^2\delta(q+mg)\delta_{q,-ng} \tag{62}$$

Next, putting it all together, let's us plug the expression for $\mathcal{S}_{12}$ in Eq. (62) into our expression for the linear interaction energy density $u$ in Eq. (42):

$$u = 2\pi\bar{\sigma}^2\sum_{n,m=-\infty}^{\infty}(-1)^{n-m}\cos\left[\frac{n\phi_s}{2}\right]\cos\left[\frac{m\phi_s}{2}\right]\cos[n\phi_1 - m\phi_2]\times\int dq\,\mathcal{W}_{n,m}(q,R,a,b)\delta(q+mg)\delta_{q,-ng} \tag{63}$$

Using the Dirac delta function to take the integral over $q$:

$$u = 2\pi\bar{\sigma}^2\sum_{n,m=-\infty}^{\infty}(-1)^{n-m}\cos\left[\frac{n\phi_s}{2}\right]\cos\left[\frac{m\phi_s}{2}\right]\times\cos[n\phi_1 - m\phi_2]\,\mathcal{W}_{n,m}(-mg,R,a,b)\delta_{-mg,-ng} \tag{64}$$

The Kronecker delta imposes that $n = m$:

$$u = 2\pi\bar{\sigma}^2\sum_{n=-\infty}^{\infty}\cos^2\left[\frac{n\phi_s}{2}\right]\cos[n(\phi_1 - \phi_2)]\,\mathcal{W}_{n,n}(-ng,R,a,b) \tag{65}$$

We can use the symmetry of the summand to obtain:

$$u = 4\pi\bar{\sigma}^2\sum_{n=0}^{\infty}\frac{\tilde{P}(n)^2}{\delta_{n,0}+1}\,\mathcal{W}_{n,n}(-ng,R,a,b)\cos[n(\phi_1 - \phi_2)] \tag{66}$$

We can write this in an even more compact form, as:

$$u = a_0 + \sum_{n=1}^{\infty}a_n(R)\cos[n(\phi_1 - \phi_2)] \tag{67}$$

Where the prefactors are defined as:

$$a_0(R) = 2\pi\bar{\sigma}^2(1-\Theta)^2\mathcal{W}_{0,0}(0,R,a,b) \tag{68}$$

$$a_{n\geq 1}(R) = 4\pi\bar{\sigma}^2\tilde{P}^2(n)\mathcal{W}_{n,n}(ng,R,a,b) \tag{69}$$

It should be noticed that Eq. (67) presents an alternating series which sum converges. The alternation in sign comes from the definition of $W_{n,n}$ (see Eq. (39)).

Finally, it remains to calculate $\mathcal{W}_{0,0}(0,R,a,b)$ and $\mathcal{W}_{n,n}(ng,R,a,b)$ for the specific choice of non-local solvent response model we used in the main text. For details of integral calculation please see Appendix A.

### 3. Uncorrelated sequences of ds-DNA molecules

The interaction between two identical parallel DNA molecules is given by Eq. (67), and generally depends on the difference in angles $\phi_1 - \phi_2$. Each such angle $\phi_i(z)$ is the consequence of an accumulation of angle increments $\{\Omega_i\}$ between each two adjacent base-pairs, separated by a base-pair rise distance of $\delta z = h \approx 3.4$ Å. The value of $\Omega_i$ generally varies from one base-pair rise to another since it is base-pair identity dependent. For identical molecules, which are characterized by a complete correlation between base-pair sequences, the value $\phi_1 - \phi_2$ remains the same throughout the length of both molecules. However, for non-correlated sequences, the value of $\phi_1 - \phi_2$ generally changes with the $z$ coordinate along the length of the molecules. To write each $\phi_i(z)$ explicitly, we first need to consider two independent boundary conditions which come about from the ability of each molecule to rotate around its long axis freely. The first is the coordinate $z = l$ for which the difference in angles $\phi_1 - \phi_2$ is kept constant. From that point the random mismatches of $\Omega_i$ start to accumulate (this is equivalent to the lamp post of the drunken person performing a random walk). The second boundary condition is the specific constant value for the difference in angles at $z = l$, i.e., $\xi = \phi_1(l) - \phi_2(l)$. Given these two parameters, the change in angle $\delta\phi(z) = \phi_2(z) - \phi_1(z)$ is given by:

$$\delta\phi(z) = \begin{cases} \xi + \sum_{j=\frac{z}{h}}^{\frac{l}{h}} \left(\Omega_2^{(j)} - \Omega_1^{(j)}\right) & z < l \\ \xi + \sum_{j=\frac{l}{h}}^{\frac{z}{h}} \left(\Omega_2^{(j)} - \Omega_1^{(j)}\right) & z > l \end{cases} \tag{70}$$

The angle increment $\Omega_i$, is modeled here as a biased random walk with mean $\mu \approx 34°$ and variance $\sigma^2 \equiv (\Delta\Omega)^2 \approx 0.0049 - 0.01$, and is distributed the same for both molecule 1 and 2. For a large number of steps, i.e. $\frac{z}{h} \gg 1$, we may approximate, according to the central limit theorem, the sum over each $\Omega_i$ as a Gaussian variable. Using Gaussian variables characteristics, we find that $\delta\phi(z)$ is distributed as a Gaussian with mean $\xi$ and variance $2\frac{|z-l|}{h}(\Delta\Omega)^2$. Lastly, $n\delta\phi$ is also a gaussian variable distributed as $n\delta\phi$ with $n\xi$ mean and variance of $2\frac{|z-l|}{h}n^2(\Delta\Omega)^2$.

Neglecting end-effects, the average total energy is given by:

$$\langle U\rangle = \int_0^L \langle u(z)\rangle dz = L\int_0^L \frac{1}{L}(a_0 + a_1\langle\cos\delta\phi\rangle + a_2\langle\cos 2\delta\phi\rangle + \cdots)dz = L\sum_{n=0}^{\infty} a_n(R)\nu_n(L) \tag{71}$$

where we defined:

$$\nu_n(L) = \frac{1}{L}\int_0^L dz\langle\cos\big(n\delta\phi(z)\big)\rangle \tag{72}$$

Since a Gaussian variable $X$ with mean $\mu$ and variance $\sigma^2$ satisfies $\langle\cos X\rangle = e^{-\frac{1}{2}\sigma^2}\cos\mu$, we have:

$$\langle\cos\big(n\delta\phi(z)\big)\rangle = \cos(n\xi)\, e^{-n^2\frac{|l-z|}{\lambda_c}} \tag{73}$$

where $\lambda_c = \frac{h}{(\Delta\Omega)^2}$ is the helical coherence length. Plugging in Eq. (73) into Eq. (72) and solving the integral we get:

$$\nu_n(\xi, l; L) = \frac{\lambda_c}{n^2 L}\left(2 - e^{-n^2\frac{l}{\lambda_c}} - e^{-n^2\frac{(L-l)}{\lambda_c}}\right)\cos(n\xi) \tag{74}$$

The optimal choice for $l$ and $\xi$ can be estimated by a two-dimensional minimisation of energy. With respect to these boundary parameters, there are two stationary points to $\frac{\langle U\rangle}{L}$. The first is $\xi = 0, \bar{x} = 0$ and the second is $\xi = \pm\arccos\left(\frac{|a_1|}{a_2}\frac{1-e^{-\frac{\bar{L}}{2}}}{1-e^{-2\bar{L}}}\right)$, $\bar{x} = 0$. The latter option is the minimum when $\frac{|a_1|}{a_2}\frac{1-e^{-\frac{\bar{L}}{2}}}{1-e^{-2\bar{L}}} \leq 1$, and the former option is a minimum whenever $\frac{|a_1|}{a_2}\frac{1-e^{-\frac{\bar{L}}{2}}}{1-e^{-2\bar{L}}} > 1$.

## 4. Homology Recognition Well

We wish to compute the energy of interaction between the two sliding homologs in a juxtaposition window of length $L$. Same as in the last section, we need to consider the two boundary conditions, namely where mismatch accumulation starts $z = D$ and what is the value of difference in angles at that point $\xi = \phi_2(D) - \phi_1(D)$. For a displacement shift $x$ of one homolog relative to the other, the change in long axis angles is given by

$$\delta\phi(z) = \delta\phi(D) + \begin{cases} -\frac{1}{h}\int_z^D\big(\Delta\Omega(z'-x) - \Delta\Omega(z')\big)dz' & 0 < z < D \\ +\frac{1}{h}\int_D^z\big(\Delta\Omega(z'-x) - \Delta\Omega(z')\big)dz' & D < z < L \end{cases} \tag{75}$$

where we made use of a continuum form which satisfies the Gaussian statistics $\Delta\Omega(z')\Delta\Omega(z'') = h(\Delta\Omega)^2\delta(z'-z'')$. The mean interaction energy is given by:

$$\langle U\rangle = \int_0^L\langle u(z)\rangle dz = L\sum_{n=0}^{\infty} a_n(R)\nu_n(x, L) \tag{76}$$

where

$$\nu_n(x, L) = \frac{1}{L}\int_0^L\langle\cos n\delta\phi\rangle dz \text{ and } n\delta\phi(x, z) = n\big(\phi_1(z) - \phi_2(x, z)\big). \tag{77}$$

Using Gaussian statistics

$$\langle\cos\big(\delta\phi(x,z)\big)\rangle = \cos\delta\phi(D)\, e^{-\frac{1}{2}\langle(\delta\phi(x,z)-\delta\phi(D))^2\rangle} \equiv \cos\delta\phi(D)\,\mu_n(x,z). \quad (78)$$

Let us proceed in calculating $\mu_n(x,z)$, or, more specifically $\langle\big(\delta\phi(z)-\delta\phi(D)\big)^2\rangle$. We shall do so separately for each region $0<x<D$ and $D<x<L$. For each region we further subdivide into subregions $0<z<D$ and $D<z<L$.

For $0<x<D$, and $0<z<D$ we have:

$$\frac{h}{(\Delta\Omega)^2}\langle\big(\delta\phi(z)-\delta\phi(D)\big)^2\rangle = \frac{1}{(\Delta\Omega)^2 h}\int_z^D\int_z^D dz'dz''\langle\big(\Delta\Omega(z'-x)-\Delta\Omega(z')\big)\big(\Delta\Omega(z''-x)-\Delta\Omega(z'')\big)\rangle$$

$$= \int_z^D\int_z^D dz'dz''\left(2\delta(z'-z'')-\delta\big(z'-(x+z'')\big)-\delta\big(z'-(z''-x)\big)\right) \quad (79)$$

Integrating term by term carefully we get

$$\frac{h}{(\Delta\Omega)^2}\langle\big(\delta\phi(z)-\delta\phi(D)\big)^2\rangle = \begin{cases} 2x & z<D-x \\ 2(D-z) & z>D-x \end{cases} \quad (80)$$

For $D<z<L$, we get:

$$h\frac{\langle(\delta\phi(z)-\langle\delta\phi(z)\rangle)^2\rangle}{(\Delta\Omega)^2} = \int_D^z\int_D^z dz'dz''\left(2\delta(z'-z'')-\delta\big(z'-(x+z'')\big)-\delta\big(z'-(z''-x)\big)\right) \quad (81)$$

which, after careful integration gives:

$$h\frac{\langle(\delta\phi(z)-\langle\delta\phi(z)\rangle)^2\rangle}{(\Delta\Omega)^2} = \begin{cases} 2(z-D) & z<D+x \\ z-D+(2x-z+D)\theta(L-x-D) & z>D+x \end{cases} \quad (82)$$

Calculating $\mu_1$ and $\mu_2$ for this region, we get:

$$\mu_1(x,L) = \frac{\lambda_c}{L}\left(\frac{D-x}{\lambda_c}e^{-\frac{x}{\lambda_c}} + 2 - e^{-\frac{x}{\lambda_c}} - e^{\frac{D}{\lambda_c}}e^{-\frac{(D+x)\theta(L-x-D)+L(1-\theta(L-x-D))}{\lambda_c}} + \theta(L-x-D)\frac{L-D-x}{\lambda_c}e^{-\frac{x}{\lambda_c}}\right) \quad (83)$$

$$\mu_2(x,L) = \frac{\lambda_c}{L}\left(\frac{D-x}{\lambda_c}e^{-4\frac{x}{\lambda_c}} + \frac{1}{2} - \frac{1}{4}\left(e^{-4\frac{x}{\lambda_c}} + e^{-\frac{4}{\lambda_c}(L-D+(D+x-L)\theta(L-x-D))}\right) + \theta(L-x-D)e^{-\frac{4x}{\lambda_c}}\frac{L-D-x}{\lambda_c}\right) \quad (84)$$

A similar calculation was performed for the region $D<x<L$ giving:

$$\mu_1(x,L) = \frac{\lambda_c}{L}\left(2 - e^{-\frac{D}{\lambda_c}} - e^{-\frac{(D+x-L)\theta(L-x-D)+L-D}{\lambda_c}} + \theta(L-x-D)\frac{L-D-x}{\lambda_c}e^{-\frac{x}{\lambda_c}}\right) \quad (85)$$

$$\mu_2(x,L) = \frac{\lambda_c}{L}\left(\frac{1}{2} - \frac{1}{4}\left(e^{-\frac{4D}{\lambda_c}} + e^{\frac{4D}{\lambda_c}}e^{-4\frac{(D+x)\theta(L-x-D)+L(1-\theta(L-x-D))}{\lambda_c}}\right) + \theta(L-x-D)\frac{L-D-x}{\lambda_c}e^{-4\frac{x}{\lambda_c}}\right) \quad (86)$$

Overall, we get the following interaction energy:

$$\frac{\langle U(0\le x\le D)\rangle - a_0 L}{\lambda_c} = a_1\cos(\delta\phi)\left(\frac{D-x}{\lambda_c}e^{-\frac{x}{\lambda_c}} + 2 - e^{-\frac{x}{\lambda_c}} - e^{-\frac{(D+x-L)\theta(L-x-D)+L-D}{\lambda_c}} + \theta(L-x-D)\frac{L-D-x}{\lambda_c}e^{-\frac{x}{\lambda_c}}\right) +$$
$$a_2\cos(2\delta\phi)\left(\frac{D-x}{\lambda_c}e^{-4\frac{x}{\lambda_c}} + \frac{1}{2} - \frac{1}{4}\left(e^{-4\frac{x}{\lambda_c}} + e^{-\frac{4}{\lambda_c}(L-D+(D+x-L)\theta(L-x-D))}\right) + \theta(L-x-D)e^{-\frac{4x}{\lambda_c}}\frac{L-D-x}{\lambda_c}\right) \quad (87)$$

$$\frac{\langle U(D\le x\le L)\rangle - a_0 L}{\lambda_c} = a_1\cos(\delta\phi)\left(2 - e^{-\frac{D}{\lambda_c}} - e^{-\frac{(D+x-L)\theta(L-x-D)+L-D}{\lambda_c}} + \theta(L-x-D)\frac{L-D-x}{\lambda_c}e^{-\frac{x}{\lambda_c}}\right) +$$
$$a_2\cos\big(2\delta\phi(D)\big)\left(\frac{1}{2} - \frac{1}{4}\left(e^{-\frac{4D}{\lambda_c}} + e^{\frac{4D}{\lambda_c}}e^{-4\frac{(D+x)\theta(L-x-D)+L(1-\theta(L-x-D))}{\lambda_c}}\right) + \theta(L-x-D)\frac{L-D-x}{\lambda_c}e^{-4\frac{x}{\lambda_c}}\right) \quad (88)$$

The optimal values for $D$ and $\xi$ which give out a minimum energy are: $D^* = L/2$ and

$$\xi^* = \begin{cases} \pm \arccos\left(\frac{a_1\mu_1(x,L)}{4a_2\mu_2(x,L)}\right) & \left|\frac{a_1\mu_1(x,L)}{4a_2\mu_2(x,L)}\right| \leq 1 \\ 0 & \left|\frac{a_1\mu_1(x,L)}{4a_2\mu_2(x,L)}\right| > 1 \end{cases} \quad (89)$$

## 5. Debye-Bjerrum Approximation

Under physiological conditions, many biological macromolecules with a high density of surface charges (DNA and chromatin in particular) are surrounded by an ionic atmosphere with Debye length $\lambda_D \approx 7$ Å. Hence, we expect to observe non-linear screening of the fixed surface charges by the ions in the electrolyte, which we can treat with the mean-field non-linear Poisson-Boltzmann model. However, the majority of the counterions that contribute to the non-linear screening reside in a thin layer around each molecule and are referred to as *condensed counterions*. We can estimate the thickness of this layer as:

$$d_c \lesssim \frac{A}{4\pi\ell_B} \quad (90)$$

where $A$ is the average area per elementary charge of the molecular surface and $\ell_B = \frac{e^2}{4\pi\varepsilon_0\varepsilon_r k_B T} \approx 7$ Å is the Bjerrum length in water. For most biological molecules, $A < 100$ Å$^2$, and therefore $d_c < 2$ Å. Within a layer of this thickness, a mean-field treatment is not appropriate. Hence, we replace the Poisson-Boltzmann approximation by explicit treatment of condensed counterions. We do this by treating this non-linear screening layer as an infinitesimally thin surface containing the fixed surface charges as well as chemisorbed ions and condensed, mobile counterions. Hence, this surface may have an arbitrary, inhomogeneous charge density, which we can define as we wish. The diffuse ionic atmosphere outside of this surface lies within the Debye-Hückel approximation. This model is accurate when $d_c$ is small compared to all other characteristic lengths in the system (for example, the surface-to-surface distance between molecules, helical pitch, the Debye length etc.)

The approach used here is similar to the Debye-Bjerrum model used in polyelectrolyte theory at non-vanishing salt concentrations, as well as the theory of concentrated electrolyte solutions, which includes the theory of Coulomb criticality, and has proved to be successful.

## Appendix A: Analytical calculation of integrals in a nonlocal electrolyte

Within the expressions derived for the electrostatic interaction energy, there are two integrals that require calculation, $\Omega_{n,m}$ and $\mathcal{A}_m$. As these will depend on the specific response model used, we begin by writing the Green's function for a nonlocal Lorentzian solvent

$$\tilde{G}\left(\sqrt{K^2 + q^2}\right) = \frac{4\pi}{(K^2+q^2)\varepsilon_s\left(\sqrt{K^2+q^2}\right)+\varepsilon\kappa^2} \quad (A1)$$

where $\kappa^{-1}$ is the Debye length, and the dielectric function is given by

$$\varepsilon_s(k) = \varepsilon_* + \frac{\varepsilon - \varepsilon_*}{1 + \frac{\varepsilon}{\varepsilon_*}\Lambda^2 k^2} \tag{A2}$$

where $\varepsilon \approx 80$, $\varepsilon_* \approx 5$ is the short range dielectric constant, and $\Lambda \approx 3$ Å is the correlation length. Hence, the integrals read

$$\Omega_{n,m}(q,x,y,z) = 4\pi yz \int_0^\infty K\, dK\, \frac{J_{n-m}(Kx) J_n(Ky) J_m(Kz)}{(K^2+q^2)\varepsilon_s\left(\sqrt{K^2+q^2}\right) + \varepsilon\kappa^2} \tag{A3}$$

$$\mathcal{A}_m(x,y,q) = \int_0^\infty K\, dK\, \frac{J_m(Kx) J_m(Ky)}{(K^2+q^2)\varepsilon_s\left(\sqrt{K^2+q^2}\right) + \varepsilon\kappa^2} \tag{A4}$$

Complex analysis of the integrands shows that the poles of both functions are the same, and imaginary described by the characteristic wavenumbers $\tilde{Q}_1$ and $\tilde{Q}_2$, given below

$$\tilde{Q}_1 = \frac{1}{\sqrt{2}}\sqrt{2q^2 + \xi\kappa^2 + \frac{1}{\Lambda^2}\left(1 + \sqrt{(1 - 2\kappa\Lambda + \xi\kappa^2\Lambda^2)(1 + 2\kappa\Lambda + \xi\kappa^2\Lambda^2)}\right)} \tag{A5}$$

$$\tilde{Q}_2 = \frac{1}{\sqrt{2}}\sqrt{2q^2 + \xi\kappa^2 + \frac{1}{\Lambda^2}\left(1 - \sqrt{(1 - 2\kappa\Lambda + \xi\kappa^2\Lambda^2)(1 + 2\kappa\Lambda + \xi\kappa^2\Lambda^2)}\right)} \tag{A6}$$

Where $\xi = \varepsilon/\varepsilon_*$, and so the solution of both integrals will follow the same procedure. Hence, we focus on $\Omega_{n,m}$ in this appendix. Knowing the dielectric function and the poles, we can rewrite $\Omega_{n,m}$ as:

$$\Omega_{n,m}(q,x,y,z) = \frac{4\pi yz}{\varepsilon\Lambda^2}\int_0^\infty K dK\, \frac{1+\xi\Lambda^2(K^2+q^2)}{(K+i\tilde{Q}_1)(K-i\tilde{Q}_1)(K+i\tilde{Q}_2)(K-i\tilde{Q}_2)} \mathcal{J}_{n-m}(Kx)\mathcal{J}_n(Ky)\mathcal{J}_m(Kz) \tag{A7}$$

Noticing the limits, we cannot simply extend the contour of integration to $-\infty$. Rather, we can consider the following integral instead, replacing $K$ with the complex number $Z$,

$$\Omega^C_{n,m}(q,x,y,z) = \int_0^\infty Z dZ\, \frac{1+\xi\Lambda^2(Z^2+q^2)}{(Z+i\tilde{Q}_1)(Z-i\tilde{Q}_1)(Z+i\tilde{Q}_2)(Z-i\tilde{Q}_2)} \mathcal{H}^{(2)}_{n-m}(Zx)\mathcal{J}_n(Zy)\mathcal{J}_m(Zz) \tag{A8}$$

where $\mathcal{H}^{(2)}_\nu(x)$ is the Hankel function of the second kind, such that $\Omega_{n,m} = \frac{4\pi yz}{\varepsilon\Lambda^2}\mathrm{Re}\{\Omega^C_{n,m}\}$. Here, we note that $x > y + z$, which determines our choice of Bessel function to convert to a Hankel function. We take the following contour:

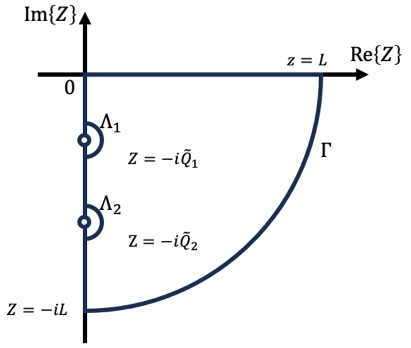


Such that

$$\oint f(z)dz = \int_0^L + \int_\Gamma + \int_{\Lambda_2} + \int_{\Lambda_1} + \int_{z\in i\mathbb{R}} = 0 \tag{A9}$$

And

$$\Omega^{C}_{n,m}(q,x,y,z) = \lim_{L\to\infty} \int_0^L = -\lim_{L\to\infty} \left\{ \int_\Gamma + \int_{\Lambda_2} + \int_{\Lambda_1} + \int_{z\in i\mathbb{R}} \right\} \tag{A10}$$

Note that when we take the real part of this integral, we can ignore the integral over $z \in i\mathbb{R}$. Additionally, the integral over the arc $\Gamma$ will tend to zero as $L \to \infty$. Hence we focus on the integrals over $\Lambda_1$ and $\Lambda_2$.

First considering the pole around which the path $\Lambda_1$ goes, we can write:

$$\int_{\Lambda_1} = \lim_{\epsilon\to 0} \int_{-i\tilde{Q}_1-\epsilon}^{-i\tilde{Q}_1+\epsilon} Z\, dZ \frac{[1+\xi\Lambda^2(Z^2+q^2)]\mathcal{H}_{n-m}(Zx)\mathcal{J}_n(Zy)\mathcal{J}_m(Zz)}{(Z+i\tilde{Q}_1)(Z-i\tilde{Q}_1)(Z+i\tilde{Q}_2)(Z-i\tilde{Q}_2)} \tag{A11}$$

Solving this integral using the substitution $Z = \epsilon e^{i\phi} - i\tilde{Q}_1$, $dZ = i\epsilon e^{i\phi} d\phi$, we obtain

$$\int_{\Lambda_1} = \frac{\pi i}{2} \tilde{g}_1 \mathcal{H}_{n-m}[-i\tilde{Q}_1 x] \mathcal{J}_n[-i\tilde{Q}_1 y] \mathcal{J}_m[-i\tilde{Q}_1 z] \tag{A12}$$

where

$$\tilde{g}_1 = \frac{\xi\Lambda^2\tilde{Q}^2_{1,\,q=0}-1}{\sqrt{(1-2\kappa\Lambda+\xi\kappa^2\Lambda^2)(1+2\kappa\Lambda+\xi\kappa^2\Lambda^2)}} \tag{A13}$$

Using the relationships between the Hankel and Bessel function with the modified Bessel functions, namely $\mathcal{J}_n(ix) = i^n I_n(x)$, $I_n(-x) = (-1)^n I_n(x)$ and $K_n(x) = \frac{\pi}{2}(-1)^{n+1}\mathcal{H}_n(-ix)$, we obtain

$$\int_{\Lambda_1} = -\Lambda^2 \tilde{g}_1 (-1)^m K_{n-m}(\tilde{Q}_1 x) I_n(\tilde{Q}_1 y) I_m(\tilde{Q}_1 z) \tag{A14}$$

Following a similar procedure, the path $\Lambda_2$ yields the following result

$$\int_{\Lambda_2} = -\Lambda^2 \tilde{g}_2 (-1)^m K_{n-m}(\tilde{Q}_2 x) I_n(\tilde{Q}_2 y) I_m(\tilde{Q}_2 z) \tag{A15}$$

where

$$\tilde{g}_2 = \frac{1-\xi\Lambda^2\tilde{Q}^2_{2,q=0}}{\sqrt{(1-2\kappa\Lambda+\xi\kappa^2\Lambda^2)(1+2\kappa\Lambda+\xi\kappa^2\Lambda^2)}} \tag{A16}$$

Putting this all together, and using $\Omega_{n,m} = \frac{4\pi yz}{\varepsilon\Lambda^2}\mathrm{Re}\{\Omega^C_{n,m}\}$, we find for $\Omega_{n,m}$

$$\Omega_{n,m}(q,x,y,z) = \frac{4\pi yz}{\varepsilon}(-1)^m\left[\tilde{g}_1 K_{n-m}(\tilde{Q}_1 x) I_n(\tilde{Q}_1 y) I_m(\tilde{Q}_1 z) + \tilde{g}_2 K_{n-m}(\tilde{Q}_2 x) I_n(\tilde{Q}_2 y) I_m(\tilde{Q}_2 z)\right] \tag{A17}$$

Where $x > y + z$.

We can do the same with $\mathcal{A}_m$ to find

$$\mathcal{A}_m(x,y,q) = \begin{cases} \frac{4\pi}{\varepsilon}\left[\tilde{g}_1 K_m(\tilde{Q}_1 x) I_m(\tilde{Q}_1 y) + \tilde{g}_2 K_m(\tilde{Q}_2 x) I_m(\tilde{Q}_2 y)\right], & x > y \\ \frac{4\pi}{\varepsilon}\left[\tilde{g}_1 K_m(\tilde{Q}_1 y) I_m(\tilde{Q}_1 x) + \tilde{g}_2 K_m(\tilde{Q}_2 y) I_m(\tilde{Q}_2 x)\right], & x < y \end{cases} \tag{A18}$$

Thus when we calculate $\partial\mathcal{A}_m/\partial y$, we must be careful to choose the correct case as above.

## Appendix B: Interaction energy of homogeneous cylinders in a Debye-Hückel medium

For Debye-Hückel media, the transformed Green's function is given by:

$$\tilde{G}\left(\sqrt{K^2+q^2}\right) = \frac{4\pi}{\epsilon_s(K^2+q^2+\kappa^2)} \tag{B1}$$

which, upon plugging into $\mathcal{W}_{n,m}(q, R_1, R)$ gives:

$$\mathcal{W}_{n,m}(q, R_1, R) = \frac{4\pi}{\epsilon_s}\int K\, dK \;\; \frac{J_m(Ka)J_n(KR_1)J_{n-m}(KR)}{(K^2+q^2+\kappa^2)} \tag{B2}$$

Which results in:

$$\mathcal{W}_{n,m}(q, R_1, R) = \frac{4\pi}{\epsilon_s} K_{n-m}(\kappa_{\text{eff}}R) I_n(\kappa_{\text{eff}}R_1) I_m(\kappa_{\text{eff}}a) \tag{B3}$$

where $\kappa_{\text{eff}} = \sqrt{\kappa^2 + q^2}$ and $I_m(x)$ and $K_m(x)$ are, correspondingly, the m[th] order modified Bessel functions of the first and second kinds.

The function $\mathcal{S}_{12}$ is given by:

$$\mathcal{S}_{12}(q, n, m) = \lim_{L\to\infty} \frac{\tilde{\sigma}_1(-q,-n)\tilde{\sigma}_2(q,m)}{L} \tag{B4}$$

$$\sigma_\nu(z, \phi_\nu) = \sigma_0 \tag{B5}$$

$$\sigma(q, n) = \frac{\sigma_0}{2\pi}\int_{-\infty}^{\infty} dz\, e^{iqz} \int_0^{2\pi} d\phi\; e^{in\phi} \tag{B6}$$

which is recognised as:

$$\sigma(q, n) = 2\pi\sigma_0\delta(q)\delta_{n,0} \tag{B7}$$

$$\mathcal{S}_{12}(q, n, m) = \lim_{L\to\infty} \frac{4\pi^2}{L}\sigma_0^2\delta(q)\delta(-q)\delta_{n,0}\delta_{-m,0} \tag{B8}$$

Using

$$\frac{\delta_{-q,0}}{2\pi} = \lim_{L\to\infty}\frac{2\pi\delta(-q)}{L} \tag{B9}$$

we get:

$$\mathcal{S}_{12}(q, n, m) = 2\pi\sigma_0^2\delta(q)\delta_{-q,0}\delta_{n,0}\delta_{-m,0} \tag{B10}$$

Plugging into $u$:

$$u = \frac{8\pi^2a^2\sigma_0^2}{\epsilon_s} K_0(\kappa R) I_0^2(\kappa a) \tag{B11}$$
